# Supplementary material for: Early detection of Crossfire attacks using deep learning
Source: arXiv:1801.00235 source file (2018-04-20)
Supplement: Supplementary file 1 [file appendix.tex]

\Huge{\textbf{Appendix Section}}
\newline

\textbf{Curriculum Vitae of Authors: }
\bigskip

Saurabh Misra
\newline

Mengxuan Tan
\newline

Mostafa Rezazad
\newline

Ngai-Man Cheung
